# Supplementary material for: An Extensive Experimental Evaluation of Automated Machine Learning Methods for Recommending Classification Algorithms (Extended Version)
Source: arXiv:2009.07430 source file (2020-09-16)
Supplement: Supplementary file 1 [file appB_activeTestingSetup.tex]

%-----------------------------------------------
%-----------------------------------------------
\newpage
\section{Active Testing and Pairwise Curve Comparison Algorithms Setup}
\label{sec:app-activeTesting}

\setcounter{table}{0}

% Data table
% latex table generated in R 3.3.0 by xtable 1.8-2 package
% Thu Nov 10 13:52:15 2016
 \begin{table}[h!]
    \tiny
    \centering
    \caption{\texttt{OpenML} datasets (1 to 57) used to train Active Testing and Pairwise Curve Comparison algorithms. For each dataset are presented: the \texttt{OpenML} id, the dataset name, the number of instances, features, classes and the majority class size.}
    \label{tab:at_algos_part1}
    \begin{tabular*}{\textwidth}
	{@{\extracolsep{\fill}}cclrrrr}
    \toprule
        \multirow{2}{*}{No} & OpenML & Name & Number of & Number of & Number of & Majority \\ 
        & data id & & Instances & Features & Classes & Class size \\
    \midrule
      1 & 3 & kr-vs-kp & 3196 &  37 &   2 & 1669 \\ 
      2 &  11 & balance-scale & 625 &   5 &   3 & 288 \\ 
      3 &  14 & mfeat-fourier & 2000 &  77 &  10 & 200 \\ 
      4 &  16 & mfeat-karhunen & 2000 &  65 &  10 & 200 \\ 
      5 &  18 & mfeat-morphological & 2000 &   7 &  10 & 200 \\ 
      6 &  21 & car & 1728 &   7 &   4 & 1210 \\ 
      7 &  22 & mfeat-zernike & 2000 &  48 &  10 & 200 \\ 
      8 &  23 & cmc & 1473 &  10 &   3 & 629 \\ 
      9 &  28 & optdigits & 5620 &  65 &  10 & 572 \\ 
      10 &  30 & page-blocks & 5473 &  11 &   5 & 4913 \\ 
      11 &  31 & credit-g & 1000 &  21 &   2 & 700 \\ 
      12 &  36 & segment & 2310 &  20 &   7 & 330 \\ 
      13 &  37 & diabetes & 768 &   9 &   2 & 500 \\ 
      14 &  40 & sonar & 208 &  61 &   2 & 111 \\ 
      15 &  44 & spambase & 4601 &  58 &   2 & 2788 \\ 
      16 &  48 & tae & 151 &   6 &   3 &  52 \\ 
      17 &  50 & tic-tac-toe & 958 &  10 &   2 & 626 \\ 
      18 &  53 & heart-statlog & 270 &  14 &   2 & 150 \\ 
      19 &  54 & vehicle & 846 &  19 &   4 & 218 \\ 
      20 &  59 & ionosphere & 351 &  35 &   2 & 225 \\ 
      21 &  60 & waveform-5000 & 5000 &  41 &   3 & 1692 \\ 
      22 &  61 & iris & 150 &   5 &   3 &  50 \\ 
      23 & 164 & molecular-biology\_promoters & 106 &  59 &   2 &  53 \\ 
      24 & 182 & satimage & 6430 &  37 &   6 & 1531 \\ 
      25 & 187 & wine & 178 &  14 &   3 &  71 \\ 
      26 & 292 & Australian & 690 &  15 &   2 & 383 \\ 
      27 & 307 & vowel & 990 &  13 &  11 &  90 \\ 
      28 & 311 & oil\_spill & 937 &  50 &   2 & 896 \\ 
      29 & 333 & monks-problems-1 & 556 &   7 &   2 & 278 \\ 
      30 & 334 & monks-problems-2 & 601 &   7 &   2 & 395 \\ 
      31 & 335 & monks-problems-3 & 554 &   7 &   2 & 288 \\ 
      32 & 336 & SPECT & 267 &  23 &   2 & 212 \\ 
      33 & 337 & SPECTF & 349 &  45 &   2 & 254 \\ 
      34 & 338 & grub-damage & 155 &   9 &   4 &  49 \\ 
      35 & 375 & JapaneseVowels & 9961 &  15 &   9 & 1614 \\ 
      36 & 446 & prnn\_crabs & 200 &   8 &   2 & 100 \\ 
      37 & 448 & analcatdata\_boxing1 & 120 &   4 &   2 &  78 \\ 
      38 & 450 & analcatdata\_lawsuit & 264 &   5 &   2 & 245 \\ 
      39 & 458 & analcatdata\_authorship & 841 &  71 &   4 & 317 \\ 
      40 & 461 & analcatdata\_creditscore & 100 &   7 &   2 &  73 \\ 
      41 & 463 & backache & 180 &  33 &   2 & 155 \\ 
      42 & 464 & prnn\_synth & 250 &   3 &   2 & 125 \\ 
      43 & 469 & analcatdata\_dmft & 797 &   5 &   6 & 155 \\ 
      44 & 475 & analcatdata\_germangss & 400 &   6 &   4 & 100 \\ 
      45 & 679 & rmftsa\_sleepdata & 1024 &   3 &   4 & 404 \\ 
      46 & 685 & visualizing\_livestock & 130 &   3 &   5 &  26 \\ 
      47 & 694 & diggle\_table\_a2 & 310 &   9 &   9 &  41 \\ 
      48 & 714 & fruitfly & 125 &   5 &   2 &  76 \\ 
      49 & 715 & fri\_c3\_1000\_25 & 1000 &  26 &   2 & 557 \\ 
      50 & 716 & fri\_c3\_100\_50 & 100 &  51 &   2 &  62 \\ 
      51 & 717 & rmftsa\_ladata & 508 &  11 &   2 & 286 \\ 
      52 & 719 & veteran & 137 &   8 &   2 &  94 \\ 
      53 & 720 & abalone & 4177 &   9 &   2 & 2096 \\ 
      54 & 721 & pwLinear & 200 &  11 &   2 & 103 \\ 
      55 & 723 & fri\_c4\_1000\_25 & 1000 &  26 &   2 & 547 \\ 
      56 & 724 & analcatdata\_vineyard & 468 &   4 &   2 & 260 \\ 
      57 & 725 & bank8FM & 8192 &   9 &   2 & 4885 \\

    \bottomrule
\end{tabular*}
\end{table}

  \begin{table}[h!]
    \tiny
    \centering
    \caption{\texttt{OpenML} datasets (58 to 122) used to train Active Testing and Pairwise Curve Comparison algorithms. For each dataset are presented: the \texttt{OpenML} id, the dataset name, the number of instances, features, classes and the majority class size.}
    \label{tab:at_algos_part2}
    \begin{tabular*}{\textwidth}
	{@{\extracolsep{\fill}}cclrrrr}
    \toprule
        \multirow{2}{*}{No} & OpenML & Name & Number of & Number of & Number of & Majority \\ 
        & data id & & Instances & Features & Classes & Class size \\
    \midrule  
      58 & 728 & analcatdata\_supreme & 4052 &   8 &   2 & 3081 \\ 
      59 & 730 & fri\_c1\_250\_5 & 250 &   6 &   2 & 131 \\
      60 & 732 & fri\_c0\_250\_50 & 250 &  51 &   2 & 133 \\ 
      61 & 733 & machine\_cpu & 209 &   7 &   2 & 153 \\ 
      62 & 735 & cpu\_small & 8192 &  13 &   2 & 5715 \\ 
    
      63 & 736 & visualizing\_environmental & 111 &   4 &   2 &  58 \\
      64 & 737 & space\_ga & 3107 &   7 &   2 & 1566 \\ 
      65 & 740 & fri\_c3\_1000\_10 & 1000 &  11 &   2 & 560 \\ 
      66 & 741 & rmftsa\_sleepdata & 1024 &   3 &   2 & 515 \\ 
      67 & 743 & fri\_c1\_1000\_5 & 1000 &   6 &   2 & 543 \\ 
      68 & 744 & fri\_c3\_250\_5 & 250 &   6 &   2 & 141 \\ 
      69 & 745 & auto\_price & 159 &  16 &   2 & 105 \\ 
      70 & 746 & fri\_c1\_250\_25 & 250 &  26 &   2 & 143 \\ 
      71 & 747 & servo & 167 &   5 &   2 & 129 \\ 
      72 & 748 & analcatdata\_wildcat & 163 &   6 &   2 & 116 \\ 
      73 & 749 & fri\_c3\_500\_5 & 500 &   6 &   2 & 263 \\ 
      74 & 750 & pm10 & 500 &   8 &   2 & 254 \\ 
      75 & 751 & fri\_c4\_1000\_10 & 1000 &  11 &   2 & 560 \\ 
      76 & 752 & puma32H & 8192 &  33 &   2 & 4128 \\ 
      77 & 753 & wisconsin & 194 &  33 &   2 & 104 \\ 
      78 & 754 & fri\_c0\_100\_5 & 100 &   6 &   2 &  54 \\ 
      79 & 756 & autoPrice & 159 &  16 &   2 & 105 \\ 
      80 & 761 & cpu\_act & 8192 &  22 &   2 & 5715 \\ 
      81 & 762 & fri\_c2\_100\_10 & 100 &  11 &   2 &  55 \\ 
      82 & 763 & fri\_c0\_250\_10 & 250 &  11 &   2 & 125 \\ 
      83 & 764 & analcatdata\_apnea3 & 450 &   4 &   2 & 395 \\ 
      84 & 765 & analcatdata\_apnea2 & 475 &   4 &   2 & 411 \\ 
      85 & 766 & fri\_c1\_500\_50 & 500 &  51 &   2 & 262 \\ 
      86 & 767 & analcatdata\_apnea1 & 475 &   4 &   2 & 414 \\ 
      87 & 768 & fri\_c3\_100\_25 & 100 &  26 &   2 &  55 \\ 
      88 & 769 & fri\_c1\_250\_50 & 250 &  51 &   2 & 137 \\ 
      89 & 770 & strikes & 625 &   7 &   2 & 315 \\ 
      90 & 772 & quake & 2178 &   4 &   2 & 1209 \\ 
      91 & 773 & fri\_c0\_250\_25 & 250 &  26 &   2 & 126 \\ 
      92 & 774 & disclosure\_x\_bias & 662 &   4 &   2 & 345 \\ 
      93 & 775 & fri\_c2\_100\_25 & 100 &  26 &   2 &  57 \\ 
      94 & 776 & fri\_c0\_250\_5 & 250 &   6 &   2 & 125 \\ 
      95 & 778 & bodyfat & 252 &  15 &   2 & 128 \\ 
      96 & 779 & fri\_c1\_500\_25 & 500 &  26 &   2 & 267 \\ 
      97 & 783 & fri\_c3\_100\_10 & 100 &  11 &   2 &  60 \\ 
      98 & 784 & newton\_hema & 140 &   4 &   2 &  70 \\ 
      99 & 788 & triazines & 186 &  61 &   2 & 109 \\ 
      100 & 792 & fri\_c2\_500\_5 & 500 &   6 &   2 & 298 \\ 
      101 & 793 & fri\_c3\_250\_10 & 250 &  11 &   2 & 135 \\ 
      102 & 794 & fri\_c2\_250\_25 & 250 &  26 &   2 & 139 \\ 
      103 & 795 & disclosure\_x\_tampered & 662 &   4 &   2 & 335 \\ 
      104 & 796 & cpu & 209 &   8 &   2 & 156 \\ 
      105 & 797 & fri\_c4\_1000\_50 & 1000 &  51 &   2 & 560 \\ 
      106 & 799 & fri\_c0\_1000\_5 & 1000 &   6 &   2 & 503 \\ 
      107 & 803 & delta\_ailerons & 7129 &   6 &   2 & 3783 \\ 
      108 & 805 & fri\_c4\_500\_50 & 500 &  51 &   2 & 264 \\ 
      109 & 806 & fri\_c3\_1000\_50 & 1000 &  51 &   2 & 555 \\ 
      110 & 807 & kin8nm & 8192 &   9 &   2 & 4168 \\ 
      111 & 812 & fri\_c1\_100\_25 & 100 &  26 &   2 &  53 \\ 
      112 & 813 & fri\_c3\_1000\_5 & 1000 &   6 &   2 & 563 \\ 
      113 & 814 & chscase\_vine2 & 468 &   3 &   2 & 256 \\ 
      114 & 816 & puma8NH & 8192 &   9 &   2 & 4114 \\ 
      115 & 818 & diggle\_table\_a2 & 310 &   9 &   2 & 165 \\ 
      116 & 819 & delta\_elevators & 9517 &   7 &   2 & 4785 \\ 
      117 & 820 & chatfield\_4 & 235 &  13 &   2 & 142 \\ 
      118 & 824 & fri\_c1\_500\_10 & 500 &  11 &   2 & 274 \\ 
      119 & 825 & boston\_corrected & 506 &  21 &   2 & 283 \\ 
      120 & 826 & sensory & 576 &  12 &   2 & 337 \\ 
      121 & 827 & disclosure\_x\_noise & 662 &   4 &   2 & 333 \\ 
      122 & 829 & fri\_c1\_100\_5 & 100 &   6 &   2 &  55 \\

    \bottomrule
\end{tabular*}
\end{table}
 
 \begin{table}[h!]
    \tiny
    \centering
    \caption{\texttt{OpenML}\texttt{OpenML} datasets (123 to 187) used to train Active Testing and Pairwise Curve Comparison algorithms. For each dataset are presented: the \texttt{OpenML}\texttt{OpenML} id, the dataset name, the number of instances, features, classes and the majority class size.}
    \label{tab:at_algos_part3}
    \begin{tabular*}{\textwidth}
	{@{\extracolsep{\fill}}cclrrrr}
    \toprule
        \multirow{2}{*}{No} & OpenML & Name & Number of & Number of & Number of & Majority \\ 
        & data id & & Instances & Features & Classes & Class size \\
    \midrule  
    
        123 & 830 & fri\_c2\_250\_10 & 250 &  11 &   2 & 159 \\ 
      124 & 832 & fri\_c3\_250\_25 & 250 &  26 &   2 & 139 \\ 
      125 & 833 & bank32nh & 8192 &  33 &   2 & 5649 \\ 
      126 & 837 & fri\_c1\_1000\_50 & 1000 &  51 &   2 & 547 \\ 
      127 & 838 & fri\_c4\_500\_25 & 500 &  26 &   2 & 284 \\ 
      128 & 841 & stock & 950 &  10 &   2 & 488 \\ 
      129 & 845 & fri\_c0\_1000\_10 & 1000 &  11 &   2 & 509 \\ 
      130 & 847 & wind & 6574 &  15 &   2 & 3501 \\ 
      131 & 849 & fri\_c0\_1000\_25 & 1000 &  26 &   2 & 503 \\ 
      132 & 850 & fri\_c0\_100\_50 & 100 &  51 &   2 &  51 \\ 
      133 & 853 & housing & 506 &  14 &   2 & 297 \\ 
      134 & 855 & fri\_c4\_500\_10 & 500 &  11 &   2 & 276 \\ 
      135 & 863 & fri\_c4\_250\_10 & 250 &  11 &   2 & 133 \\ 
      136 & 866 & fri\_c2\_1000\_50 & 1000 &  51 &   2 & 582 \\ 
      137 & 867 & visualizing\_livestock & 130 &   3 &   2 & 105 \\ 
      138 & 868 & fri\_c4\_100\_25 & 100 &  26 &   2 &  54 \\ 
      139 & 869 & fri\_c2\_500\_10 & 500 &  11 &   2 & 286 \\ 
      140 & 870 & fri\_c1\_500\_5 & 500 &   6 &   2 & 267 \\ 
      141 & 871 & pollen & 3848 &   6 &   2 & 1924 \\ 
      142 & 872 & boston & 506 &  14 &   2 & 297 \\ 
      143 & 873 & fri\_c3\_250\_50 & 250 &  51 &   2 & 142 \\ 
      144 & 875 & analcatdata\_chlamydia & 100 &   4 &   2 &  81 \\ 
      145 & 876 & fri\_c1\_100\_50 & 100 &  51 &   2 &  56 \\ 
      146 & 877 & fri\_c2\_250\_50 & 250 &  51 &   2 & 137 \\ 
      147 & 879 & fri\_c2\_500\_25 & 500 &  26 &   2 & 304 \\ 
      148 & 880 & mu284 & 284 &  11 &   2 & 142 \\ 
      149 & 884 & fri\_c0\_500\_5 & 500 &   6 &   2 & 251 \\ 
      150 & 885 & transplant & 131 &   4 &   2 &  83 \\ 
      151 & 886 & no2 & 500 &   8 &   2 & 251 \\ 
      152 & 888 & fri\_c0\_500\_50 & 500 &  51 &   2 & 256 \\ 
      153 & 889 & fri\_c0\_100\_25 & 100 &  26 &   2 &  50 \\ 
      154 & 890 & cloud & 108 &   8 &   2 &  76 \\ 
      155 & 896 & fri\_c3\_500\_25 & 500 &  26 &   2 & 280 \\ 
      156 & 900 & chscase\_census6 & 400 &   7 &   2 & 235 \\ 
      157 & 903 & fri\_c2\_1000\_25 & 1000 &  26 &   2 & 563 \\ 
      158 & 904 & fri\_c0\_1000\_50 & 1000 &  51 &   2 & 510 \\ 
      159 & 906 & chscase\_census5 & 400 &   8 &   2 & 207 \\ 
      160 & 907 & chscase\_census4 & 400 &   8 &   2 & 206 \\ 
      161 & 908 & chscase\_census3 & 400 &   8 &   2 & 208 \\ 
      162 & 909 & chscase\_census2 & 400 &   8 &   2 & 203 \\ 
      163 & 910 & fri\_c1\_1000\_10 & 1000 &  11 &   2 & 564 \\ 
      164 & 911 & fri\_c2\_250\_5 & 250 &   6 &   2 & 140 \\ 
      165 & 912 & fri\_c2\_1000\_5 & 1000 &   6 &   2 & 584 \\ 
      166 & 913 & fri\_c2\_1000\_10 & 1000 &  11 &   2 & 580 \\ 
      167 & 914 & balloon & 2001 &   3 &   2 & 1519 \\ 
      168 & 915 & plasma\_retinol & 315 &  14 &   2 & 182 \\ 
      169 & 916 & fri\_c3\_100\_5 & 100 &   6 &   2 &  56 \\ 
      170 & 917 & fri\_c1\_1000\_25 & 1000 &  26 &   2 & 546 \\ 
      171 & 918 & fri\_c4\_250\_50 & 250 &  51 &   2 & 135 \\ 
      172 & 920 & fri\_c2\_500\_50 & 500 &  51 &   2 & 295 \\ 
      173 & 922 & fri\_c2\_100\_50 & 100 &  51 &   2 &  58 \\ 
      174 & 923 & visualizing\_soil & 8641 &   5 &   2 & 4753 \\ 
      175 & 924 & humandevel & 130 &   4 &   2 &  65 \\ 
      176 & 925 & visualizing\_galaxy & 323 &   5 &   2 & 175 \\ 
      177 & 926 & fri\_c0\_500\_25 & 500 &  26 &   2 & 255 \\ 
      178 & 931 & disclosure\_z & 662 &   4 &   2 & 348 \\ 
      179 & 932 & fri\_c4\_100\_50 & 100 &  51 &   2 &  56 \\ 
      180 & 933 & fri\_c4\_250\_25 & 250 &  26 &   2 & 136 \\ 
      181 & 934 & socmob & 1156 &   6 &   2 & 900 \\ 
      182 & 935 & fri\_c1\_250\_10 & 250 &  11 &   2 & 140 \\ 
      183 & 936 & fri\_c3\_500\_10 & 500 &  11 &   2 & 272 \\ 
      184 & 937 & fri\_c3\_500\_50 & 500 &  51 &   2 & 282 \\ 
      185 & 941 & lowbwt & 189 &  10 &   2 &  99 \\ 
      186 & 943 & fri\_c0\_500\_10 & 500 &  11 &   2 & 259 \\ 
      187 & 947 & arsenic-male-bladder & 559 &   5 &   2 & 535 \\ 
  
    \bottomrule
\end{tabular*}
\end{table}

\begin{table}[h!]
    \tiny
    \centering
    \caption{\texttt{OpenML} datasets (188 to 239) used to train Active Testing and Pairwise Curve Comparison algorithms. For each dataset are presented: the \texttt{OpenML} id, the dataset name, the number of instances, features, classes and the majority class size.}
    \label{tab:at_algos_part4}
    \begin{tabular*}{\textwidth}
	{@{\extracolsep{\fill}}cclrrrr}
    \toprule
        \multirow{2}{*}{No} & OpenML & Name & Number of & Number of & Number of & Majority \\ 
        & data id & & Instances & Features & Classes & Class size \\
    \midrule  
      
      188 & 948 & quake & 2178 &   4 &   2 & 1209 \\ 
      189 & 949 & arsenic-female-bladder & 559 &   5 &   2 & 479 \\ 
      190 & 950 & arsenic-female-lung & 559 &   5 &   2 & 540 \\ 
      191 & 951 & arsenic-male-lung & 559 &   5 &   2 & 546 \\ 
      192 & 955 & tae & 151 &   6 &   2 &  99 \\ 
      193 & 956 & molecular-biology\_promoters & 106 &  59 &   2 &  72 \\ 
      194 & 958 & segment & 2310 &  20 &   2 & 1980 \\ 
      195 & 962 & mfeat-morphological & 2000 &   7 &   2 & 1800 \\ 
      196 & 965 & zoo & 101 &  18 &   2 &  60 \\ 
      197 & 969 & iris & 150 &   5 &   2 & 100 \\ 
      198 & 970 & analcatdata\_authorship & 841 &  71 &   2 & 524 \\ 
      199 & 971 & mfeat-fourier & 2000 &  77 &   2 & 1800 \\ 
      200 & 973 & wine & 178 &  14 &   2 & 107 \\ 
      201 & 974 & hayes-roth & 132 &   5 &   2 &  81 \\ 
      202 & 976 & kdd\_JapaneseVowels & 9961 &  15 &   2 & 8347 \\ 
      203 & 979 & waveform-5000 & 5000 &  41 &   2 & 3308 \\ 
      204 & 980 & optdigits & 5620 &  65 &   2 & 5048 \\ 
      205 & 983 & cmc & 1473 &  10 &   2 & 844 \\ 
      206 & 987 & collins & 500 &  24 &   2 & 420 \\ 
      207 & 991 & car & 1728 &   7 &   2 & 1210 \\ 
      208 & 994 & vehicle & 846 &  19 &   2 & 628 \\ 
      209 & 995 & mfeat-zernike & 2000 &  48 &   2 & 1800 \\ 
      210 & 996 & prnn\_fglass & 214 &  10 &   2 & 138 \\ 
      211 & 997 & balance-scale & 625 &   5 &   2 & 337 \\ 
      212 & 1004 & kdd\_synthetic\_control & 600 &  62 &   2 & 500 \\ 
      213 & 1006 & lymph & 148 &  19 &   2 &  81 \\ 
      214 & 1011 & ecoli & 336 &   8 &   2 & 193 \\ 
      215 & 1012 & flags & 194 &  30 &   2 & 125 \\ 
      216 & 1014 & analcatdata\_dmft & 797 &   5 &   2 & 642 \\ 
      217 & 1016 & vowel & 990 &  14 &   2 & 900 \\ 
      218 & 1020 & mfeat-karhunen & 2000 &  65 &   2 & 1800 \\ 
      219 & 1021 & page-blocks & 5473 &  11 &   2 & 4913 \\ 
      220 & 1025 & analcatdata\_germangss & 400 &   6 &   2 & 310 \\ 
      221 & 1043 & ada\_agnostic & 4562 &  49 &   2 & 3430 \\ 
      222 & 1048 & jEdit\_4.2\_4.3 & 369 &   9 &   2 & 204 \\ 
      223 & 1049 & pc4 & 1458 &  38 &   2 & 1280 \\ 
      224 & 1050 & pc3 & 1563 &  38 &   2 & 1403 \\ 
      225 & 1054 & mc2 & 161 &  40 &   2 & 109 \\ 
      226 & 1056 & mc1 & 9466 &  39 &   2 & 9398 \\ 
      227 & 1061 & ar4 & 107 &  30 &   2 &  87 \\ 
      228 & 1063 & kc2 & 522 &  22 &   2 & 415 \\ 
      229 & 1064 & ar6 & 101 &  30 &   2 &  86 \\ 
      230 & 1065 & kc3 & 458 &  40 &   2 & 415 \\ 
      231 & 1066 & kc1-binary & 145 &  95 &   2 &  85 \\ 
      232 & 1067 & kc1 & 2109 &  22 &   2 & 1783 \\ 
      233 & 1068 & pc1 & 1109 &  22 &   2 & 1032 \\ 
      234 & 1069 & pc2 & 5589 &  37 &   2 & 5566 \\ 
      235 & 1071 & mw1 & 403 &  38 &   2 & 372 \\ 
      236 & 1073 & jEdit\_4.0\_4.2 & 274 &   9 &   2 & 140 \\ 
      237 & 1075 & datatrieve & 130 &   9 &   2 & 119 \\ 
      238 & 1115 & teachingAssistant & 151 &   7 &   3 &  52 \\ 
      239 & 1121 & badges2 & 294 &  12 &   2 & 210 \\ 
    
    \bottomrule
\end{tabular*}
\end{table}

%-----------------------------------------------
%-----------------------------------------------

% Testing data

 \begin{table}[h!]
    \tiny
    \centering
    \caption{\texttt{OpenML} classification datasets used to test Active Testing and Pairwise Curve Comparison algorithms. For each dataset are presented: the \texttt{OpenML} data id, the dataset name (Name), the number of instances, features, classes and the majority class size. Datasets with no \texttt{OpenML} id are not available at \texttt{OpenML}.}
    \label{tab:at_algos_part5}
    \begin{tabular*}{\textwidth}
	{@{\extracolsep{\fill}}cclrrrr}
    \toprule
    
    \multirow{2}{*}{No} & OpenML & Name & Number of & Number of & Number of & Majority \\ 
        & data id & & Instances & Features & Classes & Class size \\
    \midrule
    1 & - & CE & 478 & 764 & 2 & 288 \\
    2 & - & DM & 119 & 585 & 2 & 80 \\
    3 & - & MM & 89 & 886 & 2 & 63 \\
    4 & - & SC & 248 & 698 & 2 & 208 \\
    5 & - & DNA3 & 139 & 332 & 2 & 106 \\
    6 & - & DNA11 & 135 & 102 & 2 & 102 \\
    7 & - & PS & 4303 & 443 & 2 & 4043 \\
    8 & - & chen-2002 & 179 & 85 & 2 & 104 \\
    9 & - & chowdary-2006 & 104 & 182 & 2 & 62 \\
    10 & - & nutt-2003-v2 & 28 & 1070 & 2 & 14 \\
    11 & - & singh-2002 & 102 & 339 & 2 & 52 \\
    12 & - & west-2001 & 49 & 1198 & 2 & 25 \\    
    13 & 1562 & dbworld-bodies &  64 & 4702 &   2 &  35 \\ 
    14 & 1561 & dbworld-bodies-stemmed &  64 & 3721 &   2 &  35 \\ 
    15 & 392 & oh0.wc & 1003 & 3182 &  10 & 194 \\       
    16 & 394 & oh5.wc & 918 & 3012 &  10 & 149 \\ 
    17 & 401 & oh10.wc & 1050 & 3238 &  10 & 165 \\ 
    18 & 386 & oh15.wc & 913 & 3100 &  10 & 157 \\ 
    19 & 391 & re0.wc & 1504 & 2886 &  13 & 608 \\ 
    20 & 395 & re1.wc & 1657 & 3758 &  25 & 371 \\ 
    \bottomrule
\end{tabular*}
\end{table}

%-----------------------------------------------
%-----------------------------------------------

% Algorithm's setupID
% latex table generated in R 3.3.2 by xtable 1.8-2 package
% Mon Mar  6 11:10:46 2017
\begin{table}[ht]
\tiny
\centering
 \caption{Algorithm configurations and their respective setup Ids evaluated in Active Testing and Pairwise Curve Comparison  methods.}
 \label{tab:setupIds}
\begin{tabular}{clcl}
  \toprule
 SetupID & Algorithm Configuration & SetupID & Algorithm Configuration \\ 
  \midrule
1 & J48\_C\_0.15\_M\_1 &  36 & JRIP\_O\_1\_N\_1 \\ 
  2 & J48\_C\_0.15\_M\_16 &  37 & JRIP\_O\_2\_N\_1 \\ 
  3 & J48\_C\_0.15\_M\_2 &  38 & JRIP\_O\_3\_N\_1 \\ 
  4 & J48\_C\_0.15\_M\_32 &  39 & JRIP\_O\_4\_N\_1 \\ 
  5 & J48\_C\_0.15\_M\_4 &  40 & JRIP\_O\_5\_N\_1 \\ 
  6 & J48\_C\_0.15\_M\_64 &  41 & JRIP\_O\_1\_N\_2 \\ 
  7 & J48\_C\_0.15\_M\_8 &  42 & JRIP\_O\_2\_N\_2 \\ 
  8 & J48\_C\_0.1\_M\_1 &  43 & JRIP\_O\_3\_N\_2 \\ 
  9 & J48\_C\_0.1\_M\_16 &  44 & JRIP\_O\_4\_N\_2 \\ 
  10 & J48\_C\_0.1\_M\_2 &  45 & JRIP\_O\_5\_N\_2 \\ 
  11 & J48\_C\_0.1\_M\_32 &  46 & JRIP\_O\_1\_N\_3 \\ 
  12 & J48\_C\_0.1\_M\_4 &  47 & JRIP\_O\_2\_N\_3 \\ 
  13 & J48\_C\_0.1\_M\_64 &  48 & JRIP\_O\_3\_N\_3 \\ 
  14 & J48\_C\_0.1\_M\_8 &  49 & JRIP\_O\_4\_N\_3 \\ 
  15 & J48\_C\_0.25\_M\_1 &  50 & JRIP\_O\_5\_N\_3 \\ 
  16 & J48\_C\_0.25\_M\_16 &  51 & JRIP\_O\_1\_N\_4 \\ 
  17 & J48\_C\_0.25\_M\_2 &  52 & JRIP\_O\_2\_N\_4 \\ 
  18 & J48\_C\_0.25\_M\_32 &  53 & JRIP\_O\_3\_N\_4 \\ 
  19 & J48\_C\_0.25\_M\_4 &  54 & JRIP\_O\_4\_N\_4 \\ 
  20 & J48\_C\_0.25\_M\_64 &  55 & JRIP\_O\_5\_N\_4 \\ 
  21 & J48\_C\_0.25\_M\_8 &  56 & JRIP\_O\_1\_N\_5 \\ 
  22 & J48\_C\_0.2\_M\_1 &  57 & JRIP\_O\_2\_N\_5 \\ 
  23 & J48\_C\_0.2\_M\_16 &  58 & JRIP\_O\_3\_N\_5 \\ 
  24 & J48\_C\_0.2\_M\_2 &  59 & JRIP\_O\_4\_N\_5 \\ 
  25 & J48\_C\_0.2\_M\_32 &  60 & JRIP\_O\_5\_N\_5 \\ 
  26 & J48\_C\_0.2\_M\_4 &  61 & BayesNet\_SCORE\_BAYES\_alpha\_0.1 \\ 
  27 & J48\_C\_0.2\_M\_64 &  62 & BayesNet\_SCORE\_BAYES\_alpha\_0.2 \\ 
  28 & J48\_C\_0.2\_M\_8 &  63 & BayesNet\_SCORE\_BAYES\_alpha\_0.3 \\ 
  29 & J48\_C\_0.3\_M\_1 &  64 & BayesNet\_SCORE\_BAYES\_alpha\_0.4 \\ 
  30 & J48\_C\_0.3\_M\_16 &  65 & BayesNet\_SCORE\_BAYES\_alpha\_0.5 \\ 
  31 & J48\_C\_0.3\_M\_2 &  66 & BayesNet\_SCORE\_MDL\_alpha\_0.1 \\ 
  32 & J48\_C\_0.3\_M\_32 &  67 & BayesNet\_SCORE\_MDL\_alpha\_0.2 \\ 
  33 & J48\_C\_0.3\_M\_4 &  68 & BayesNet\_SCORE\_MDL\_alpha\_0.3 \\ 
  34 & J48\_C\_0.3\_M\_64 &  69 & BayesNet\_SCORE\_MDL\_alpha\_0.4 \\ 
  35 & J48\_C\_0.3\_M\_8 &  70 & BayesNet\_SCORE\_MDL\_alpha\_0.5 \\ 
   \bottomrule
\end{tabular}
\end{table}

%-----------------------------------------------
%-----------------------------------------------
