# Supplementary material for: An Extensive Experimental Evaluation of Automated Machine Learning Methods for Recommending Classification Algorithms (Extended Version)
Source: arXiv:2009.07430 source file (2020-09-16)
Supplement: Supplementary file 2 [file appC_baselines_rks.tex]

%-----------------------------------------------
%-----------------------------------------------

\newpage
\section{Active Testing and Pairwise Curve Comparison Recommended Rankings}
\label{sec:app-baselines_rks}

\setcounter{table}{0}

% latex table generated in R 3.3.2 by xtable 1.8-2 package
\begin{table}[ht]
\centering
\tiny
\caption{Algorithm rankings recommended by Active Testing (1 to 60). For each dataset and training data partition it is shown the top ten algorithm configurations. The corresponding setup ids are mapped in Table~\ref{tab:setupIds}.}
\label{tab:at_rk_part1}
% [inline block 0: 6 envs, 54593 chars -> data_tex | \begin{tabular}{clcrrrrrrrrrr}   \toprule...]

\end{table}

%-----------------------------------------------
%-----------------------------------------------
